# Supplementary material for: Optimal Co-Design of a Hybrid Energy Storage System for Truck Charging
Source: arXiv:2506.01426 source file (2025-06-02)
Supplement: Supplementary file 1 [file Appendix.tex]

\appendices

\section{Parameters Values of Different Combination of ESS} \label{app:matlab_function3}
The properties of various ESS types are summarized in Table ~\ref{tab:t2}. 
These parameter values are sourced from \cite{storage}. 
\begin{table}[h]
    \centering
    \caption{Properties of different types of ESS}
    \label{tab:t2}
    \begin{adjustbox}{max width= \textwidth}

        \begin{tabular}{|p{1.4cm}|p{1cm}|p{1cm}|p{1cm}|p{1cm}|p{1cm}|p{1.2cm}|}
            \hline
            ESS Unit & Max Energy Capacity (kWh) & Max Power Capacity(kW) & Energy Cost(\euro / kWh) & Power Cost  (\euro / kW) & Charging Efficiency & Discharging Efficiency \\
            \hline
            Li-ion Batteries & 40000 & 40000 & 400 & 800 & 0.83 & 0.88 \\
            \hline
            Flywheel & 5000 & 20000 & 2800 & 310 &  0.85 & 0.95 \\
            \hline
            Sodium Sulphur Batteries & 300000 & 100000 &  675 & 595 &  0.75 & 0.85 \\
            \hline
            Super-capacitors & 20000 & 40000 & 175 &  300 & 0.95 & 0.97 \\
            \hline
            Fuelcells & 10000 & 20000 & 100 & 2979& 0.40 & 0.60 \\
            \hline
        \end{tabular}
    \end{adjustbox}
\end{table}
